# Supplementary material for: Electrically tunable artificial gauge potential for polaritons
Source: arXiv:1610.07358 ancillary file (2016-10-24)
Supplement: Supplementary file 1 [file SI.pdf]

# SUPPLEMENTARY INFORMATION

## Electrically tunable artificial gauge potential for polaritons

Hyang-Tag Lim, Emre Togan, Martin Kroner, Javier Miguel-Sanchez, and Atac Imamoğlu

*Institute of Quantum Electronics, ETH Zurich, CH-8093 Zurich, Switzerland.*

### I. SAMPLE

Our sample consists of three layers of 9.6 nm-thick $In_{0.04}Ga_{0.96}As$ quantum wells (QWs) sandwiched between two distributed Bragg reflectors (DBRs) formed by 20 (top) and 22 (bottom) pairs of $\lambda/4$ thick AlAs/GaAs layers. The GaAs spacer layer containing QWs between the top and bottom DBRs is $1\lambda$ thick. Spectral linewidths, measured at a position where the cavity mode is far red detuned from the exciton mode, indicate that the cavity has a Q factor exceeding $10^4$ (FWHM linewidth 0.11 meV). The exciton emission spectrum at the same position has a FWHM linewidth less than 1.2 meV.

Using electron beam litography and lift-off techniques we have defined rectangular metal (10 nm Ti, 210 nm Au) pads that are 700 $\mu$m $\times$ 120 $\mu$m. All of the experiments reported in this paper were carried out between two such pads that are separated by 30 $\mu$m. These pads are wire bonded onto a chip carrier, and were driven by a high voltage amplifier (Falco Systems WMA-300) to apply electric fields to the QW.

To confirm that the above pad configuration provides a uniform and controllable electric field distribution we performed a 2D electrostatic simulation of the dielectric environment in COMSOL. We modeled the AlAs/GaAs/InGaAs environment as a single dielectric with $\epsilon = 12.9$. The gates are modeled as 200 nm thick metals with a 30 $\mu$m gap, and the electric potential is constant and fixed on their boundary. The electric potential, and the electric field distribution when one of the gates is applied 1 V and the other is kept at 0 V is illustrated in Figure S1.

In the simulations we find that the electric field within a few $\mu$m from the center of the gap of the gates at a depth that corresponds to the QW position should be relatively uniform and along the $x$ direction. In this uniform region the electric field is 0.69 $V_G/(30\ \mu\text{m})$ where $V_G$ is the applied voltage between the gates.

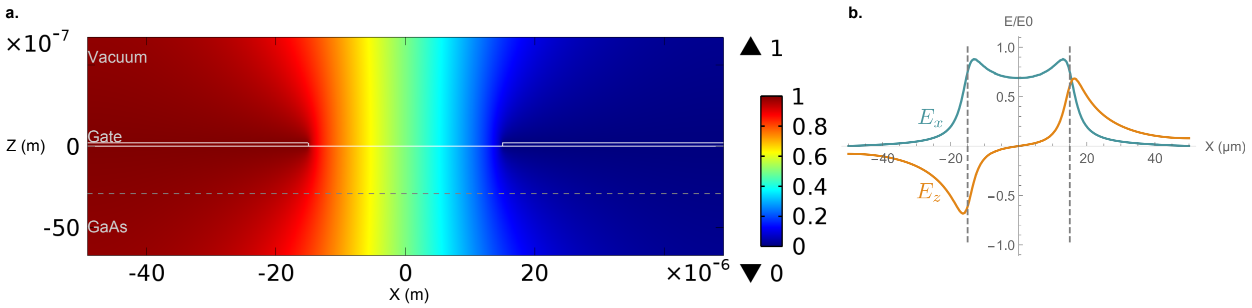


Figure S1: **Simulation of the electric field profile. a.** Calculated electric potential for 1 V applied to the left gate while the right gate is kept at 0 V. White solid lines show the boundaries of different regions containing different materials that are modeled (labeled on figure). Dashed gray line indicates the position of the electric field lines cuts. **b.** The line cut in **a** showing the electric field components at $z = -2.7\,\mu$m which corresponds to position of the QW. $E_0 = 1/30$ V/$\mu$m. Vertical gray dashed lines indicate the position of the edges of the gates.

## II. EXPERIMENTAL DETAILS

We find that in measurements where electric field is applied, the results are affected by the duration, intensity, and energy of excitation lasers. We believe these changes are due to excess charge carriers that are optically created that screen the externally applied electric field. In order to avoid such affects, in experiments where an applied electric field is needed, we perform experiments with a weak laser (New Focus TLB-6716, $<$ 100 pW for reflection experiments and $\leq$ 40 nW for interference experiments) and, to reduce light exposure further, we apply a sequence of low duty cycle laser pulses. These laser pulses are timed with a voltage pulse sequence that alternates the sign of the applied voltage between the gates to ensure that the average electric field applied to the sample remains 0.

For reflection and interference experiments we use the pulse sequence illustrated in Figure S2. To acquire reflection or interference data corresponding to a target voltage $V_{\text{target}}$ we ensure that the counter or the camera (PointGray Grasshopper 3 41C6NIR) is gated so that data from the time interval when the applied voltage is $V_{\text{target}}$ is recorded. Voltage pulse lengths are chosen to be 22.4 $\mu$s. To limit the exposure time of the laser on the sample, the excitation laser is modulated using an acousto-optic modulator (AOM, double pass, extinction $\geq$ 50 dB). The excitation laser is switched on by the AOM only around the time interval where $V_{\text{target}}$ is applied. Following

these voltage pulses we apply 20 pairs of the high voltage pulse $\pm V_{\text{high}} = \pm 10$ V to remove the remaining charge carriers created during the measurement so that these excessive charge carriers do not affect the following measurement. Our data is not sensitive to the exact values used in the sequence, for example voltage value used for $V_{\text{high}}$ pulses, the number of pairs of $V_{\text{high}}$ pulses used, voltage pulse lengths, and laser illumination duration. Hence these values can be varied without affecting the results, but some form of this pulse sequence is necessary to obtain consistent electric field dependent data. For all the electric field dependent data reported in this paper, we use the sequence described in this paragraph.

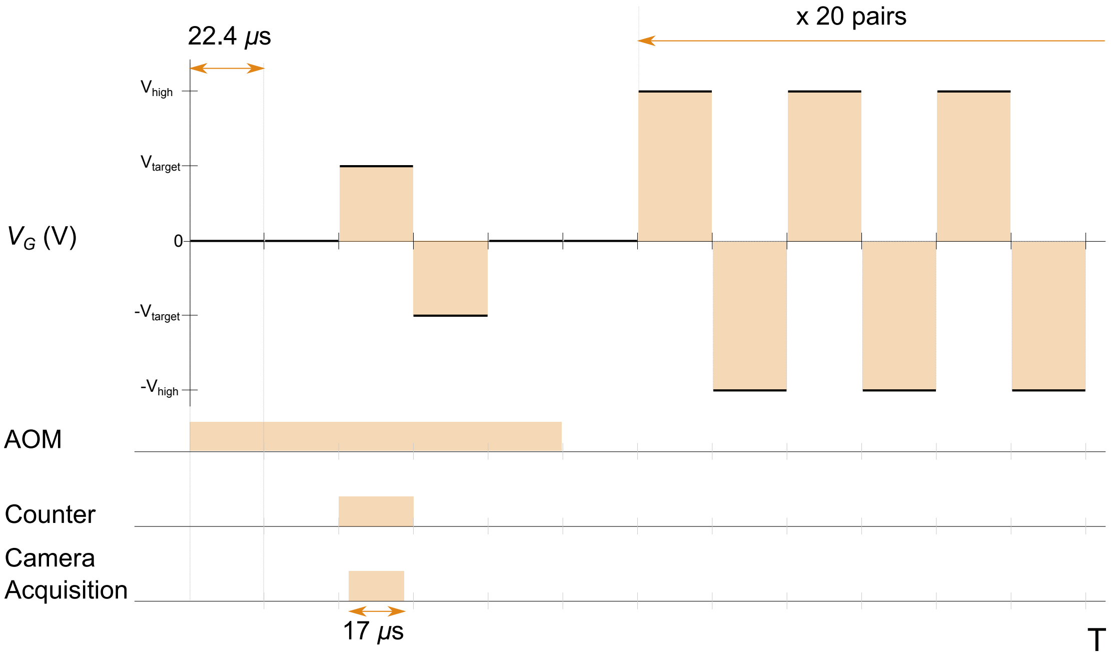


Figure S2: **Pulse sequence.** We acquire the data only when the target voltage $V_{\text{target}}$ is applied. This is ensured by timing the exposure of the camera, and gating the counter. Each voltage pulse is 22.4 $\mu$s. The laser is incident on the sample only when $V_G$ is $\pm V_{\text{target}}$ or 0.

Each data point measured presented in the main text is an average of data recorded in multiple runs of the pulse sequence. For example the reflection data shown in Figure 1 (main text) consists of 4,500 repetitions of the pulse sequence for each target voltage value, whereas the interference image shown in Figure 3 (main text) is formed by acquiring and summing 107,000 frames from the camera; each frame corresponds to a repetition of the pulse sequence. Data acquisition from the camera is carried out in blocks of 1,000 frames where pixel values from all 1,000 frames are added to form a single image. Following a block of data acquisition we do an equal acquisition with 1,000

frames with the illumination laser turned off and record the difference between the two images to remove any noise due to a persistent background in the images.

Polarization of the excitation beams is fixed to be linear (close to $p$-polarization) for all experiments. In the reflection measurement we measure the reflected light intensity without any additional polarization filtering. In polariton interference experiment the polarizer in front of the camera transmits the light nearly orthogonally polarized to the incident beams to observe high visibility interference images. This nearly orthogonal polarization configuration significantly attenuates the intensity of the reflected excitation lasers, however does not significantly attenuate the elliptically polarized emission from the polariton transitions at high magnetic fields.

## III. EXTRACTION OF POLARITON AND EXPERIMENTAL PARAMETERS

Magnetic field dependent $k$ resolved photoluminescence (PL) spectra measurements allow measurement of many parameters that allow us to accurately model the polariton behaviour at high magnetic fields [1]. To measure the $k$ resolved PL spectra, polaritons are created non-resonantly by a 780 nm continuous-wave diode laser. The incoming collimated laser beam passes through a high numerical aperture (NA) lens (NA = 0.68) so that the beam is focused on the sample plane. Then the PL signals from the sample also pass through the same lens. The back aperture of the high NA lens is the Fourier plane of emission. Emission around a particular in-plane momentum ($k_x$, $k_y$) is collected by coupling the light from a small spot in the Fourier plane into a single mode fiber which is connected to a spectrometer. To obtain the polariton energy dispersion with respect to the in-plane wavevector $k_y$, we varied the position of the single-mode fiber, which changes the collection spot on the Fourier plane. For each position that corresponds to $k_x = 0$ and a $k_y$ value we record the PL spectrum on the spectrometer. The incident 780 nm laser is blocked using a 800 nm long-pass filter at the entrance to the spectrometer.

Experimental results for the PL dispersion measurements at $B_z = 0$ T, 3 T, and 6 T are shown in Figure S3. For each $k_y$ value we fit two Lorentzian lineshapes to determine the lower polariton (LP, lower energy eigenstate) and upper polariton (UP, higher energy eigenstate) energies. We then fit the exciton-polariton energy dispersion with respect to the in-plane momentum $\hbar k_y$ to:

$$\epsilon_{LP,UP}\left(k_y\right) = \frac{1}{2}\left[\epsilon_{\text{cav}}\left(k_y\right) + \epsilon_{\text{exc}}\left(k_y\right)\right] \pm \frac{1}{2}\sqrt{\left[\epsilon_{\text{cav}}\left(k_y\right) - \epsilon_{\text{exc}}\left(k_y\right)\right]^2 + \Omega^2}, \tag{1}$$

where $\Omega$ is the exciton cavity coupling strength that we refer to as Rabi energy, and we assume that

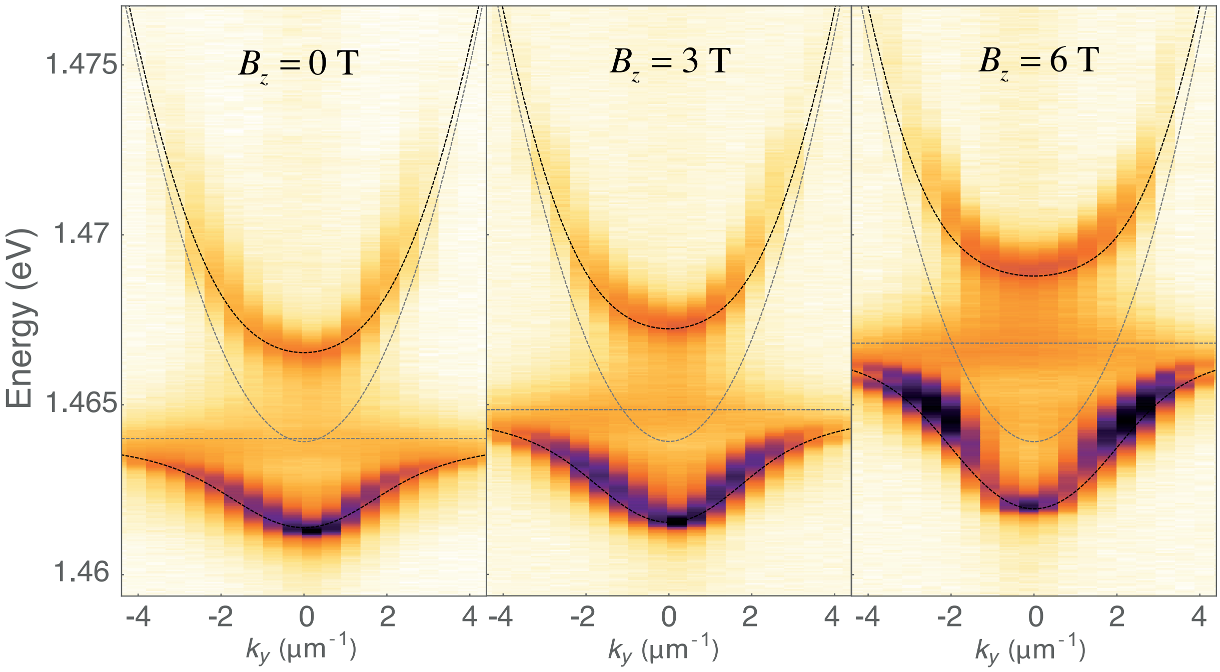


Figure S3: $k_y$ **resolved photoluminescence spectra of exciton-polaritons.** The grey dashed lines are bare cavity (curved) and exciton (flat) energy dispersion and the black dashed lines correspond to the upper and lower polariton resonances. As $B_z$ increases from 0 T to 6 T, the cavity energy remains same while the exciton energy increases due to the diamagnetic shift. Two peaks are present for lower polariton energy dispersion at high magnetic fields and large wavevectors, this we attribute to the influence of Zeeman splitting of the exciton transitions. Logarithm of the intensity of the emission is represented by the color scale.

$\epsilon_{\text{exc}}(k_y) \simeq \epsilon_{\text{exc}}(0)$ and $\epsilon_{\text{cav}}(k_y) \simeq \epsilon_{\text{cav}}(0) + \frac{1}{2m_{cav}}(\hbar k_y)^2$. Based on this relation, we can extract $\epsilon_{\text{exc}}(0)$, $\epsilon_{\text{cav}}(0)$, and $\Omega$ from the experimental result at each magnetic field, these extracted values are shown in Figure S4. We will use these values in Section IV when describing the detailed model we use to describe polariton behaviour.

### A. $k_y$ distribution of detection and excitation beams

Due to the finite size of the beams used, a $k_y$ uncertainty is present for both excitation and detection beams. With this uncertainty, we expect emission spectra measured around a mean $k_y$ value to be asymmetric, and the linewidth of the spectra to depend on this mean value. In particular our collection fiber acts as a filter and selects a distribution of $k_y$ values. We model the field distribution as a probability density function given by $f_{k_y}(k'_y) = \frac{1}{\sqrt{2\sigma_k^2\pi}} e^{-\frac{(k'_y - k_y)^2}{2\sigma_k}}$. We assume a

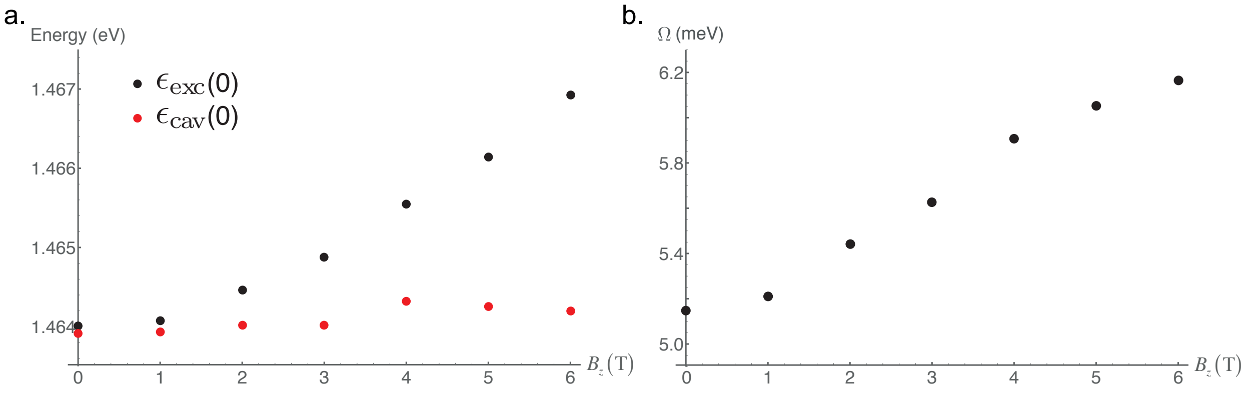


Figure S4: **Magnetic field dependence of exciton energy, cavity energy and Rabi energy. a.** The exciton energy $\epsilon_{\text{exc}}$ (black) increases with $B_z$ while the cavity mode energy $\epsilon_{\text{cav}}$ (red) is more-or-less constant regardless of $B_z$. **b.** Rabi energy $\Omega$ increases with $B_z$.

polariton resonance at $\epsilon_{LP}(k'_y)$ leads to an emission intensity lineshape given by $A\frac{\Gamma/2}{(\epsilon-\epsilon_{LP}(k'_y))^2+(\Gamma/2)^2}$ where $A$ is a constant characterizing intensity of polariton emission. The measured spectrum is then modeled by

$$I(\epsilon,k_y)=\int dk'_y|f_{k_y}(k'_y)|^2\left[A\frac{\Gamma/2}{(\epsilon-\epsilon_{LP}(k'_y))^2+(\Gamma/2)^2}\right]$$

With $\Gamma=120\,\mu\text{eV}$, $\sigma_k=0.5\times10^6\ \text{m}^{-1}$ we obtain reasonable agreement between the model and the observed lineshapes. Figure S5 illustrates the resulting asymmetric lineshapes as well as change in the expected linewidths with $k_y$. Note that at high $k_y$ values there is a high energy tail in the emission lineshapes that is not captured by this model. This tail occurs at energies close to the bare exciton resonance.

To measure the $k_y$ distribution of the excitation beams used for the interference experiment (main text Figure 3) we slightly modify the interference experiment performed. We detune the excitation laser to the red of the polariton resonances so that the laser does not excite any polaritons, and we change the polarizer angle in front of the camera such that two beams have equal detected intensities. We also change the distance between the high NA lens and the sample so that the two beams overlap at the sample surface. With the sample illuminated by the $k_y^-$ beam and the $k=0$ beam, an image of the light intensity at the surface shows an interference pattern illustrated in Figure S6. We re-emphasize that, unlike the experiments in the main text, here polaritons have not been excited, and the image purely show the interference of two laser beams. This interference pattern is due to the spatially varying phase between two beams, for simplicity (considering only

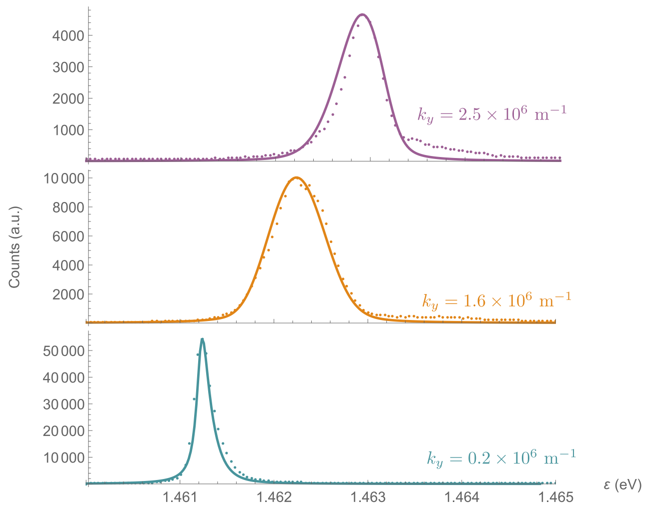


Figure S5: **Changes in PL emission lineshape with $k_y$ value.** Dots are horizontal line cuts of the data shown in Figure S3 at $B_z = 0$ T, solid lines are estimated lineshapes using $I(\epsilon, k_y)$ given in text.

$y$ direction) we model this interference as the interference of two beams that are defined by their field distributions $f_{k_y^-}(k_y')$ and $f_0(k_y')$. To extract $k_y^-$ and $\sigma_k^-$ we take a 2D Fourier Transform of the intensity image, and analyze the line cut at $k_x = 0$. From the position of the two Gaussian peaks we find $k_y^- = -2.9 \times 10^6$ m$^{-1}$. From their widths we find $\sigma_k^- = 0.4 \times 10^6$ m$^{-1}$. Acquiring and analyzing a dataset using $k_y^+$ excitation beam we find $k_y^+ = 2.7 \times 10^6$ m$^{-1}$ and $\sigma_k^+ = 0.5 \times 10^6$ m$^{-1}$.

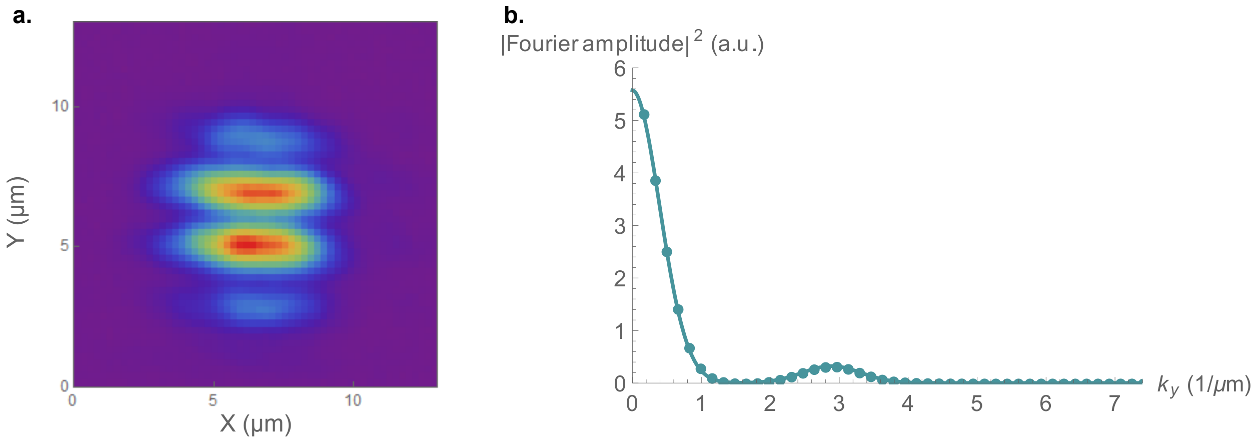


Figure S6: **Estimation of $k_y$ from interference images. a.** Interference images between the $k = 0$ beam and the $k_y^-$ beam. **b.** Line cut of the 2D Fourier Transform of the image in a, showing the positive $k_y$ values at $k_x = 0$. Solid lines are obtained by fitting a sum of two Gaussian functions one centered at $k_y = 0$ the other centered at $k_y = k_y^-$.

### B. Extracting electric field dependent energy shift of polaritons

Due to the fiber coupling we employ, the excitation laser intensity exhibits significant changes (up to 25 %) as its energy is tuned. Since the excitation intensity is less than 100 pW, we do not expect any changes in the polariton behavior due to these intensity variations. To be able to fit, and visualize the underlying changes in intensity due to excitation of polariton resonances, we calculate and plot the ratio of the recorded intensity to the average of the intensity of the data obtained for the six highest voltage values applied for each laser energy. For example in Figure 1d in the main text each horizontal line is obtained by dividing the reflected intensity for each voltage by the average intensity of the reflection at 11.04, 11.52, 12, 12.48, 12.96 and 13.44 V.

This normalization procedure however affects the lineshape of the reflection data. The procedure above (due to the Stark shift) effectively calculates the ratio by dividing by the average of data points of reflected intensity at high energy tails of the polariton resonance. If these points overlap with the tail due to the asymmetric lineshape (observed in the PL spectra, Figure S5) that extends to high energies, or overlaps with the polariton resonance, the reflection ratio at low energies can have values higher than 1. To account for this lineshape that is asymmetric in energy relative to the polariton resonance, we include a smooth step function in our fits. The fitting function we use at low magnetic field is given by :

$$R_{\text{low}}(\epsilon) = b_r + a_r \frac{(\Gamma/2)^2}{(\epsilon - \epsilon_0)^2 + (\Gamma/2)^2} + a_{\text{step}} \tanh\left(\frac{\epsilon - \epsilon_0}{\epsilon_{\text{step}}}\right).$$

We use for our fits $\epsilon_{\text{step}} = 0.2$ meV. At high magnetic fields the data exhibits two closely spaced dips that we attribute to be due to the interplay of the Zeeman splitting of the exciton transitions and the TE-TM splitting of the photonic modes, and use:

$$R_{\text{high}}(\epsilon) = b_r + a_{r,+} \frac{(\Gamma_+/2)^2}{(\epsilon - \epsilon_0 + \Delta)^2 + (\Gamma_+/2)^2} + a_{r,-} \frac{(\Gamma_-/2)^2}{(\epsilon - \epsilon_0 - \Delta)^2 + (\Gamma_-/2)^2} + a_{\text{step}} \tanh\left(\frac{\epsilon - \epsilon_0}{\epsilon_{\text{step}}}\right).$$

We expect, due to the finite TE-TM splitting at the $k_y^{\pm}$ values that we perform the measurements that the transitions will be elliptically polarized and the two dips might be of different amplitude.

## IV. MODEL OF POLARITONS UNDER MAGNETIC AND ELECTRIC FIELDS

We model the behaviour of polaritons in our system by numerically determining the eigenvalues and the associated wavefunctions of a Schrödinger equation for the excitons in the system. We

compare the measured observables obtained in various experiments with the results of calculations based on the numerical study both to extract parameters that describe the exciton system, as well as to verify the physical origin of the change in the observables.

The Hamiltonian for the 2D exciton relative motion wave function $\psi(\vec{r})$ is given by [2, 3]

$$H = -\frac{\hbar^2}{2\mu}\Delta_r + \frac{eB_z}{2\eta}\hat{L}_z + \frac{P^2}{2M} + \frac{1}{2\mu}\left(\frac{B_z}{2}\right)^2 r^2 + \frac{e}{M}\vec{P}\times(B_z\hat{z})\cdot\vec{r} + V(r) + e(E_{\text{ext}}\hat{x})\cdot\vec{r}. \quad (2)$$

where the Hamiltonian is described in SI unit and $\vec{r} = \vec{r}_e - \vec{r}_h$ is the relative coordinate, $\vec{R} = (m_e\vec{r}_e + m_h\vec{r}_h)/(m_e + m_r)$ is the center of mass (CM) coordinate, $\hat{L}_z = i\hbar\hat{z}\times\nabla_r$ is the angular momentum operator in the $z$ (growth) direction, $\vec{P} = \hbar k_y\hat{y}$ is the exciton magnetic CM momentum. Note that $\vec{P}$ is the conserved momentum of the exciton in a magnetic field and associated with translational invariance in the plane of the quantum well [2]. $E_{\text{ext}}\hat{x}$ is the applied electric field, $B_z$ the magnetic field in the growth direction, $\mu^{-1} = m_e^{-1} + m_h^{-1}$, $\eta = m_e^{-1} - m_h^{-1}$, and $M = m_e + m_h$ is the $e - h$ pair total mass (total exciton mass).

We ignore the $\frac{eB}{2\eta}\hat{L}_z$ term in Eq. (2) since we are dealing with the ground state of the 2D exciton wave function, which is spatially symmetric ($1s$ state for $B_z = 0$). We also ignore the center of mass kinetic energy term $(\hbar\vec{k})^2/(2M)$ since we fix the CM momentum $\hbar\vec{k}$ in the experiment. Thus, this term gives a constant energy shift.

The effective Coulomb potential for a QW with finite width $d$ is [4–6]

$$V(r) = -\frac{e^2}{4\pi\varepsilon\varepsilon_0}\int_0^d\int_0^d dz_e dz_h \frac{|U_e(z_e)|^2\,|U_h(z_h)|^2}{\sqrt{r^2 + (z_e - z_h)^2}}, \quad (3)$$

where $\varepsilon$ is the relative permittivity of the material, $\varepsilon_0$ is the vacuum permittivity, and we assume that the QW has infinite barriers. The wavefuntions of the electron and hole in the growth direction is given by $U_i(z_i) = \sqrt{\frac{2}{d}}\sin\left(\frac{z_i}{d}\pi\right)$ where $i$ is either $e$ or $h$. If we introduce the variable $u = (z_e - z_h)/d$ and $v = (z_e + z_h)/d$, then Eq. (3) can be written as:

$$\begin{aligned} V(r) &= -\frac{1}{\pi\varepsilon\varepsilon_0 d}\int_0^1\int_u^{2-u} dvdu \frac{\sin^2\left(\frac{u+v}{2}\pi\right)\sin^2\left(\frac{u-v}{2}\pi\right)}{\sqrt{\left(\frac{r}{d}\right)^2 + u^2}} \\ &= -\frac{1}{4\pi\varepsilon\varepsilon_0 d}\int_0^1 du \frac{(1-u)\left[2+\cos(2\pi u)\right] + \frac{3}{2\pi}\sin(2\pi u)}{\sqrt{\left(\frac{r}{d}\right)^2 + u^2}} \\ &\equiv -\frac{1}{4\pi\varepsilon\varepsilon_0}h(r). \end{aligned}$$

We use Mathematica's finite element method for numerically solving the Schrödinger equation with the Hamiltonian of Eq. (2) to obtain the energy and the wave function of the lowest energy

state. The computation region is limited to $r_{\max} = 10\ a_0$ ($0 \leq |r| \leq r_{\max}$, and $a_0 = 4\pi\varepsilon\varepsilon_0\hbar^2/\mu e^2$, 3D Bohr radius of the exciton), which is large enough that the lowest eigenvalue of the equation does not change (up to six digits) as $r_{\max}$ increases.

The physical parameter values used in this calculation are summarized in Table I. $m_0$ is the electron mass and we choose the remaining parameters such as $k_y$, $\mu$, and $M$, as we discuss below, to best match with our experimental data.

Table I: Physical parameter values

| Parameter | Symbol | Value |
|---|---|---|
| Relative permittivity (GaAs) | $\varepsilon$ | 12.9 |
| Quantum well width | $d$ | 9.6 nm |
| In-plane wavevector | $k_y^{\pm}$ | $\pm 2.8 \times 10^6\ \mathrm{m}^{-1}$ |
| Exciton effective (reduced) mass | $\mu$ | $0.04\ m_0$ |
| Total exciton mass | $M$ | $0.07\ m_0$ |
| Cavity effective mass | $m_{\mathrm{cav}}$ | $6 \times 10^{-5}\ m_0$ |

### A. Diamagnetic shift of excitons

We calculate the energy of the lowest energy eigenstate of Eq. (2) with $E_{\mathrm{ext}} = 0$ as a function of magnetic field, $B_z$, and compare the shift of energy of this state with the shift of the extracted exciton transition energy obtained in Section III. To match with the experimental results on the exciton energy change we vary the reduced mass of the exciton $\mu$. See Figure S7 for the comparison between the theory with various $\mu$ and the experimental results. Based on the results on Figure S7, we choose $\mu \sim 0.04\ m_0$. Then, the binding energy of the exciton with no external magnetic and electric field is 7.94 meV.

### B. Effect of the applied electric field on excitons

Figure S8a shows the shift of energy of the lowest energy eigenstate of Eq. (2) for $B_z = 0$ T, 3 T, and 5 T as a function of $E_{\mathrm{ext}}$. Similar to Figures 1 and 2 in the main text, the exciton energy shift can be fitted with a second order polynomial in $E_{\mathrm{ext}}$. The maximum exciton energy is obtained at $E_{\mathrm{ext}} = \tilde{E}_{\mathrm{ext}}$. The polarizability of the exciton, also, decreases as $B_z$ increases.

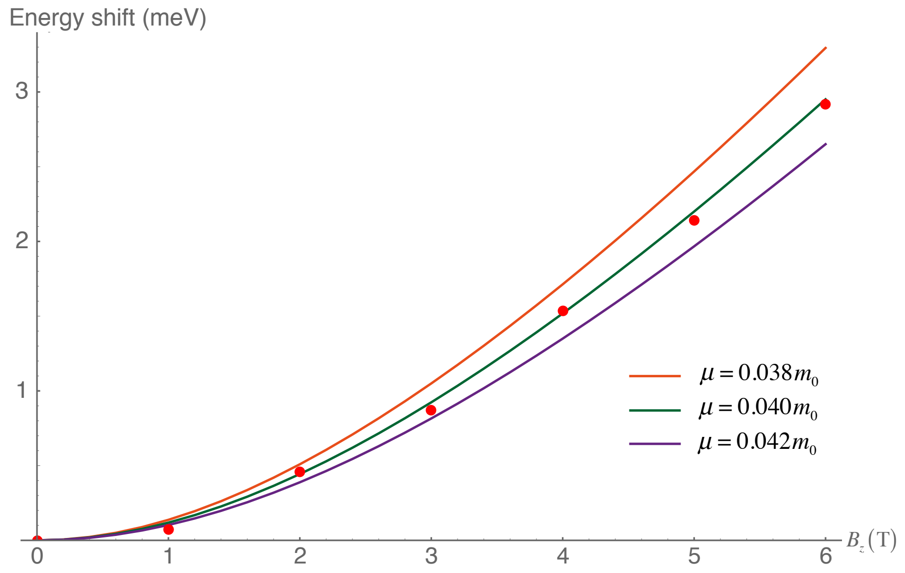


Figure S7: **Exciton diamagnetic shift.** As the magnetic field increases, the exciton energy increases. Red data points are the experimental results and the blue, yellow, and green lines are the theory lines with $\mu = 0.038 m_0,\ 0.040 m_0,\ 0.042 m_0$, respectively.

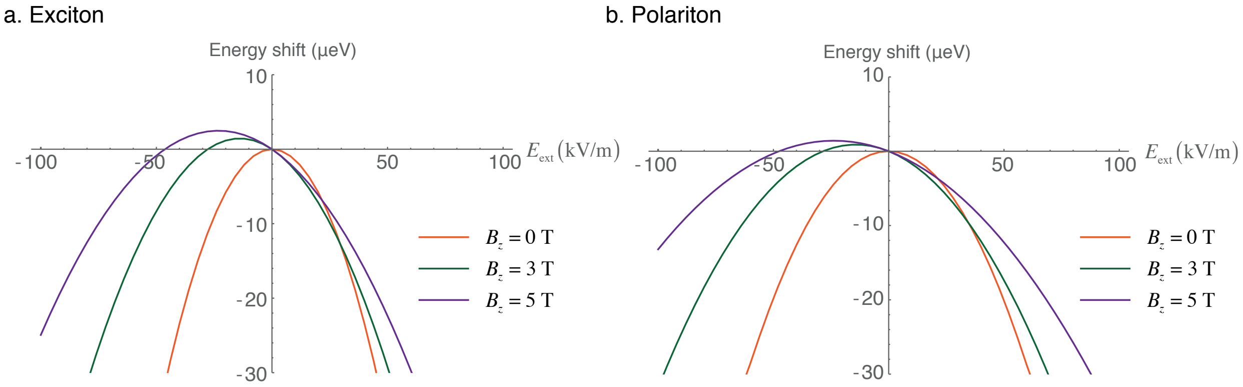


Figure S8: **Energy shift with applied electric field. a.** Exciton and **b.** Lower polariton energy shows parabolic shifts against the applied electric field $E_{\text{ext}}$. Energy of the exciton changes more rapidly than the energy of the polariton. The orange, green, and purple lines correspond to $B = 0$ T, 3 T, and 5 T, respectively. $k_y = 2.8 \times 10^6$ m$^{-1}$ and $M = 0.07\ m_0$.

### C. Effect of the magnetic field on Rabi energy

The Rabi energy $\Omega\left(B_z, E_{\text{ext}}\right)$ is proportional to the norm of the exciton wave function $\left|\psi\left(r=0\right)\right|$ [6], thus, to quantify the changes in $\Omega$ we use $\Omega\left(B_z, E_{\text{ext}}\right) = \Omega\left(B_z = 0, E_{\text{ext}} = 0\right) \frac{\left|\psi(r=0, B_z, E_{\text{ext}})\right|}{\left|\psi(r=0, B_z=0, E_{\text{ext}}=0)\right|}$. The relative Rabi energy increases with $B_z$ as shown in

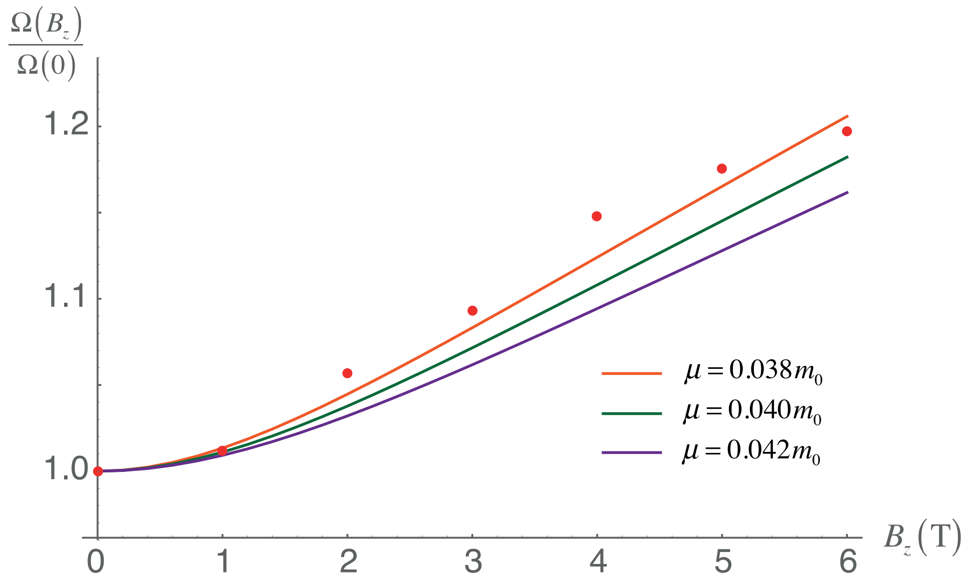


Figure S9: **Change in Rabi energy with magnetic field.** As the magnetic field increases, the Rabi energy increases. Red data points are the experimental results and the blue, yellow, and green lines are the theory lines with $\mu = 0.038m_0,\ 0.040m_0,\ 0.042m_0$, respectively.

Figure S9.

## D. Effect of the applied electric field on polaritons

Electric field alters the exciton energy thereby changing polariton resonance energy. In addition polarization of the exciton due to $E_{\text{ext}}$ reduces the electron hole overlap, leading to a reduced $\Omega$, which also changes the polariton resonance energy. To model the polariton behaviour we use Eq. (1) where $\Omega$ and $\epsilon_{\text{exc}}$ depend on both $B_z$ and $E_{\text{ext}}$. Shifts in $\epsilon_{\text{exc}}\left(B_z, E_{\text{ext}}\right)$ are found by identifying the energy shifts of the lowest energy eigenstate of Eq. (2). The cavity photon energy is given as $\epsilon_{\text{cav}}\left(k_y\right) \simeq \epsilon_{\text{cav}}\left(0\right) + \frac{\hbar^2}{2m_{\text{cav}}} k_y^2$ where we assume $E_{\text{ext}}$ or $B_z$ does not change the cavity resonance and dispersion. Changes in $\Omega$ are calculated as indicated in the previous section. Figure S8b shows the lower polariton energy shift with $E_{\text{ext}}$ at $B_z = 0$ T, 3 T, and 5 T.

We fit the polariton energy shift with $E_{\text{ext}}$ to a second order polynomial of $E_{\text{ext}}$, i.e. $\epsilon_{LP}(E_{\text{ext}}) \simeq \epsilon_{LP}(0) - \vec{d} \cdot \vec{E}_{\text{ext}} - \alpha E_{\text{ext}}^2$. The comparison between the theoretical result (both of the exciton and polariton cases) and the experiment is shown in Figure S10. Increase in $\epsilon_{LP}(0)$ with $B_z$ is less compared to the calculated increase for the exciton (Figure S10a), as the increase in $\Omega$ leads to red-shift of the LP energy.

Dependence of the polarizability $\alpha$ on $B_z$ is depicted in Figure S10b. We compare the theoretical result of $\alpha$ for polaritons with the experimental results by varying the reduction factor $\gamma$ of the applied electric field $E_{\text{ext}} = \gamma \frac{V_G}{30\ \mu\text{m}}$ where $V_G$ is the potential applied to the gate. We find good agreement with the experimental results when $\gamma = 0.84 \pm 0.01$ where the error is the fitting error. Note that the COMSOL simulation gives $\gamma \sim 0.69$ as discussed in Section I. As shown in Figure S10b, both polariton and exciton polarizabilities decrease with $B_z$ but the polarizability of the polariton is smaller than that of the exciton.

Here, as in the main text, we calculate the difference of the effective electric fields $\Delta E_{\text{eff}}$ between the case of $k_y^{\pm} = \pm 2.8 \times 10^6\ \text{m}^{-1}$, this is shown as Figure S10c. Unlike Figures S10a and b, $\Delta E_{\text{eff}}$

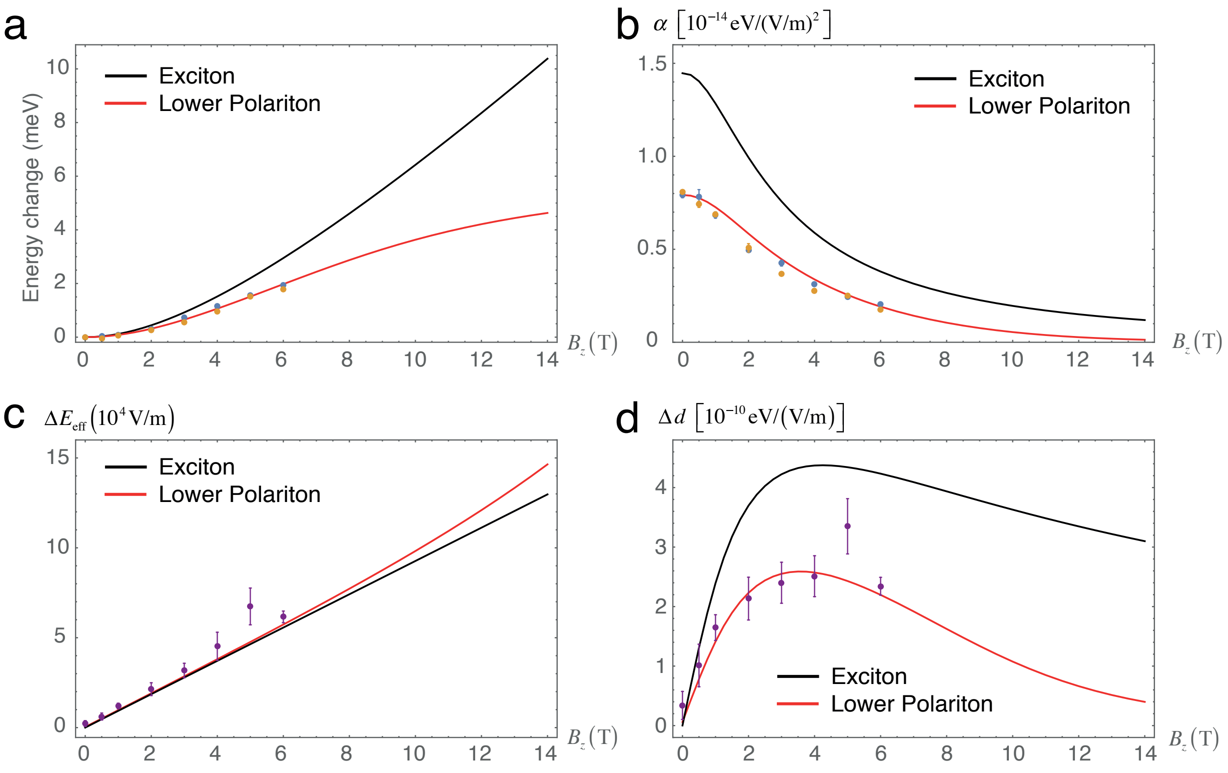


Figure S10: **Magnetic field dependence.** For each figure, the black and red lines correspond to the exciton and the polariton simulation results, respectively. The yellow and blue data points corresponds to the experimental data for the polaritons excited with $k_y^+ = 2.7 \times 10^6\ \text{m}^{-1}$ and $k_y^- = -2.9 \times 10^6\ \text{m}^{-1}$, respectively. **a.** Exciton and polariton energy at $E_{\text{ext}} = 0$ increases with $B_z$. **b.** The polarizability $\alpha$ decreases with $B_z$. **c.** Difference between the effective electric fields $\Delta E_{\text{eff}}$ for $k_y^+$ and $k_y^-$. **d.** Difference between the induced dipole moments $\Delta d$ for $k_y^+$ and $k_y^-$. For the theory lines, we used $|k_y^{\pm}| = 2.8 \times 10^6\ \text{m}^{-1}$ and $M = 0.07\ m_0$.

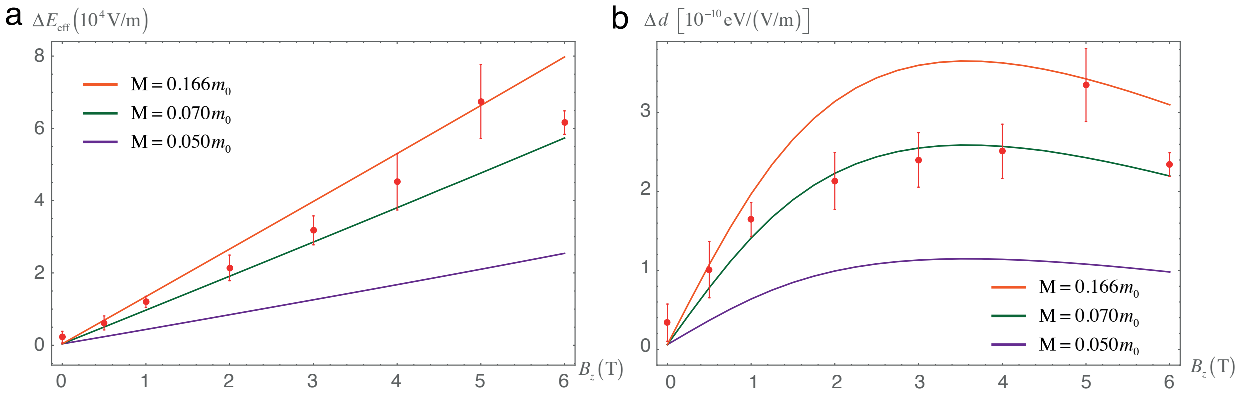


Figure S11: **Exciton total mass dependence.** The orange, green and purple lines correspond to the result with the exciton mass $M = 0.166\ m_0$, $0.07\ m_0$, and $0.05\ m_0$, respectively. **a.** Difference between the effective electric fields $\Delta E_{\rm eff}$ for $k_y^+$ and $k_y^-$. **b.** Difference between the induced dipole moments $\Delta d$ for $k_y^+$ and $k_y^-$. As $M$ increases, both of $\Delta E_{\rm eff}$ and $\Delta d$ increases. $M = 0.07\ m_0$ fits well with our experimental data.

for polariton and the exciton cases are very similar to each other and the small discrepancy is due to the fact that the Rabi energy is reduced by $E_{\rm ext}$. The electric field difference $\Delta E_{\rm eff}$ shows linear dependence on $B_z$. Note that we find that the total exciton mass $M \sim 0.07\ m_0$ gives a good agreement between the theoretical and the experimental results. See Figure S11 for the simulation results with three different $M$ values.

The difference of the induced dipole moments $\Delta d$ between $k_y^{\pm}$ with $B_z$ is shown in Figure S10d. $d$ corresponds to the induced dipole moment of the exciton or polariton due to the in-plane momentum and $B_z$. Figure S10d shows that the dipole moment of the polariton increases with $B_z$ up to around 3 - 4 T and then decreases with $B_z$ for higher magnetic fields. A remarkable feature is that the magnetic field at which the dipole moment reaches the maximum value is different for the exciton and the polariton cases, in our sample, the polariton has the maximum value around 3 - 4 T while the exciton has its maximum value around 4 - 5 T. This is due to the fact that the exciton content of the lower polariton decreases with $B_z$.

### E. Effective vector potential for polaritons

For polaritons at arbitrary detuning, it is not generally possible to write the lower (or upper) polariton dispersion as a free particle with single effective mass. However for a small range of wavevector values ($\delta k_y$) around a particular wavevector $k'_y$ ($k_y = k'_y + \delta k$) we will show that it is

possible to describe polaritons as particles moving in a vector potential. Using the description in the main text, the energy difference between the cavity mode and the exciton mode is:

$$\Delta(k_y) = \epsilon_{\text{cav}}(k_y) - \epsilon_{\text{exc}}(k_y) = \epsilon_{\text{cav}}(0) - \epsilon'_{\text{exc}}(0) + \frac{1}{2m_{\text{cav}}}(\hbar k_y)^2 - \frac{1}{2M'}(\hbar k_y - qA_{\text{eff}})^2$$

The energy eigenvalues in Eq. (1) can be re-written as:

$$\epsilon_{LP,UP}(k_y) = \frac{1}{2}\left(\Delta(k_y) \pm \sqrt{\Delta^2(k_y) + \Omega^2}\right) + \epsilon'_{\text{exc}}(0) + \frac{1}{2M'}(\hbar k_y - qA_{\text{eff}})^2$$

Assuming $k'_y \gg \delta k_y$ we do a linear expansion in $\delta k_y$ of $\epsilon_{LP}(k_y)$ and find:

$$\epsilon_{LP}(k_y) \simeq \epsilon(k'_y) + \frac{1}{2m}(\hbar k_y - qA)^2$$

where $A = \frac{m}{M} 2\alpha B_z E_x |X_k|^2$ and $\epsilon(k'_y) = \epsilon_{\text{exc}}(k'_y) + \frac{1}{2}\left(\Delta(k'_y) - \sqrt{\Delta^2(k'_y) + \Omega^2}\right) - \frac{1}{2m}\left(\hbar k'_y - qA\right)^2$, $m^{-1} = |C_k|^2 \frac{1}{m_{\text{cav}}} + |X_k|^2 \frac{1}{M'}$ with $|C_k|^2 = \frac{1}{2}\left(1 - \frac{\Delta(k'_y)}{\sqrt{\Delta^2(k'_y)+\Omega^2}}\right)$ and $|X_k|^2 = \frac{1}{2}\left(1 + \frac{\Delta(k'_y)}{\sqrt{\Delta^2(k'_y)+\Omega^2}}\right)$ the cavity and exciton Hopfield coefficients.

[1] Pietka, B. *et al.* Magnetic field tuning of exciton-polaritons in a semiconductor microcavity. *Physical Review B* **91**, 075309 (2015).

[2] Gor'kov, P. & Dzyaloshinskii, I. E. Contribution to the theory of the mott exciton in a strong magnetic field. *Soviet Physics JETP* **26**, 449–451 (1968).

[3] Lozovik, Y. E., Ovchinnikov, I. V., Volkov, S. Y., Butov, L. V. & Chemla, D. S. Quasi-two-dimensional excitons in finite magnetic fields. *Physical Review B* **65**, 235304 (2002).

[4] Kavokin, A. V. *et al.* The effect of a Coulomb well on the absorption and magnetoabsorption spectra of strained InGaAs/GaAs heterostructures. *Semiconductors* **31**, 950–960 (1997).

[5] Oliveira, C., Freire, J., Freire, V. & Farias, G. Inhomogeneous broadening arising from interface fluctuations in strained $In_xGaAs_{1-x}$/GaAs and $(In_uGaAs_{1-u})_v(InP)_{1-v}$/InP quantum wells. *Applied Surface Science* **234**, 38–44 (2004).

[6] Stepnicki, P., Pietka, B., Morier-Genoud, F., Deveaud, B. & Matuszewski, M. Analytical method for determining quantum well exciton properties in a magnetic field. *Physical Review B* **91**, 195302 (2015).
